# Supplementary material for: Substrate Effects on Spin Relaxation in Two-Dimensional Dirac Materials with Strong Spin-Orbit Coupling
Source: arXiv:2206.00784 source file (2022-12-04)
Supplement: Supplementary file 1 [file SI-Dec3.pdf]

# Supplemental Material for: Substrate Effects on Spin Relaxation in Two-Dimensional Dirac Materials with Strong Spin-Orbit Coupling

Junqing Xu[1,*] and Yuan Ping[1,†]

[1]*Department of Chemistry and Biochemistry, University of California, Santa Cruz, CA 95064, USA*

(Dated: December 4, 2022)

## SI. THE SIMULATION OF SPIN LIFETIME

Spin lifetime is calculated based on the method developed in Ref. 1. To define spin lifetime, we follow the time evolution of the observable

$$S_i\left(t\right)=\mathrm{Tr}\left[s_i\rho\left(t\right)\right], \tag{S1}$$

where $\rho\left(t\right)$ is the density matrix in the Schrödinger picture; $s_i$ is spin Pauli matrix in Blöch basis along direction $i$. This time evolution must start at an initial state (at $t = t_0$) with a net spin i.e. $\delta\rho(t_0) = \rho(t_0) - \rho^{\mathrm{eq}} \neq 0$ such that $\delta S_i(t_0) = S_i\left(t_0\right) - S_i^{\mathrm{eq}} \neq 0$, where "eq" corresponds to the final equilibrium state. We evolve the density matrix through the quantum master equation given in Ref. 1 (Eq. 5 therein) for a long enough simulation time, typically from hundreds of ps to $\mu$s, until the evolution of $S_i\left(t\right)$ can be reliably fitted by

$$S_i\left(t\right)-S_i^{\mathrm{eq}}=\left[S_i\left(t_0\right)-S_i^{\mathrm{eq}}\right]exp\left[-\frac{t-t_0}{\tau_{s,i}}\right]\times\cos\left[\Omega\left(t-t_0\right)+\phi\right]. \tag{S2}$$

to extract the relaxation time, $\tau_{s,i}$. Above, $\Omega$ is oscillation frequency due to Larmor precession. For ML-Ge systems, spins are strongly polarized along $z$ direction, so that for spin relaxation along $z$ direction, there is no Larmor precession and $\Omega$ can be safely set to zero.

In Ref. 1, we have shown that it is suitable to generate the initial spin imbalance by applying a test magnetic field at $t = -\infty$, allowing the system to equilibrate with a net spin and then turning it off suddenly at $t_0$.

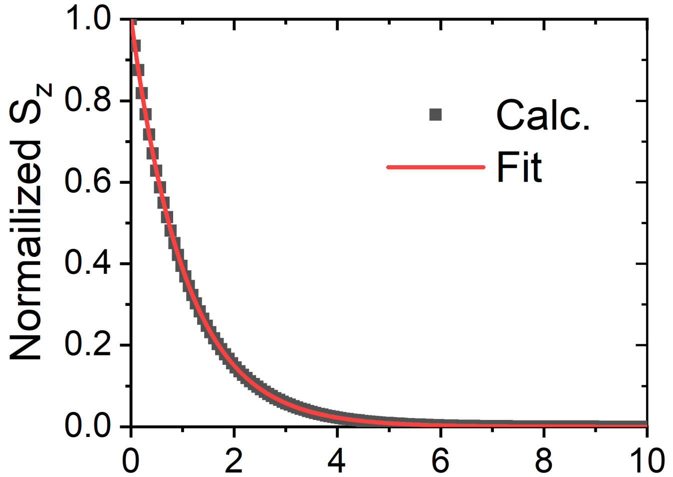


FIG. S1. Time evolution of $S_z$ of intrinsic ML-Ge-InSe holes at 50 K after the initial spin imbalance generated by a test magnetic field. "Calc." denotes calculated $S_z$. "Fit" denotes fitted $S_z$ using Eq. S2.

In Fig. S1, we compare calculated $S_z$ and fitted ones using Eq. S2 of intrinsic ML-Ge-InSe holes at 50 K after the initial spin imbalance generated by a test magnetic field. We find the fitted curve matches the calculated one perfectly, which gives spin lifetime $\tau_{s,i}$.

## SII. SPIN RELAXATION IN ML-GE WITH ONLY INTRAVALLEY SCATTERING

In this work, we define intravalley and intervalley scattering as the scattering within a single valley ($K$ or $K'$) and that between $K$ and $K'$ valleys, respectively. In this section, we will examine spin relaxation with only intravalley scattering for introducing the weight factor $w$ as defined in Ref. 2, which is related to the importance of intravalley scattering and presents in the definition of the relative intervalley spin relaxation contribution $\eta = \left(\tau_{s,z}^{\text{inter}}\right)^{-1} / \left[\left(\tau_{s,z}^{\text{inter}}\right)^{-1} + w\left(\tau_{s,z}^{\text{intra}}\right)^{-1}\right]$ in the caption of Fig. 2.

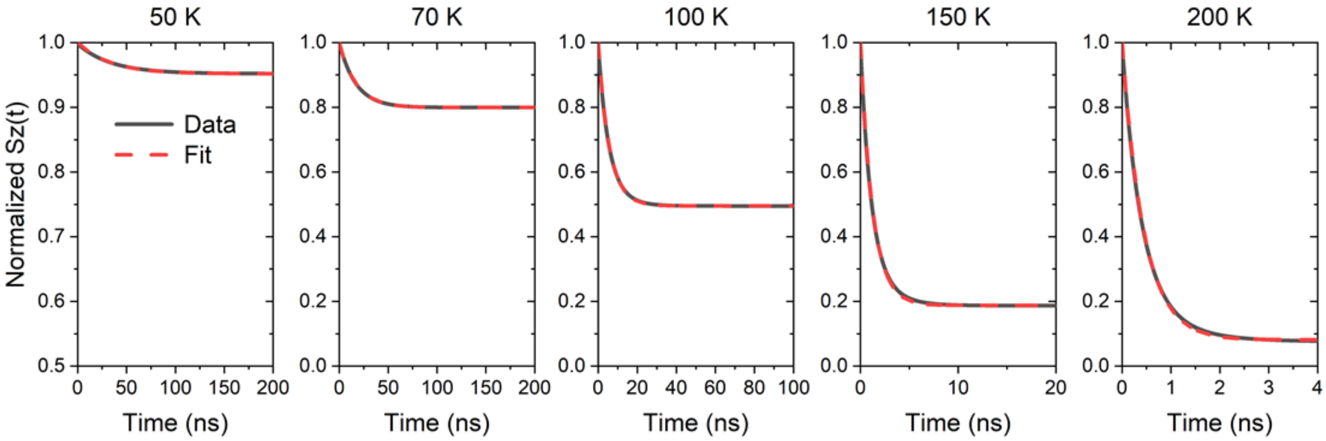


FIG. S2. Time evolution of calculated (solid black) and fitted (dashed red, Eq. S3) $S_z$ of ML-Ge under $E_z$=5 V/nm considering only intravalley scattering. Because the intervalley scattering is turned off in these calculations, the $S_z$ does not decay to zero.

From our real-time dynamics simulations, we found that when both intervalley and intravalley scatterings are included, the decay of $S_z(t)$ will be well described by Eq. S2 and $S_z$ will finally decay to zero at $t \to \infty$, as shown in Fig. S1.

However, with only intravalley scattering, since the states in $K$ valley and those in $K'$ valley are completely disconnected, the spin imbalance (along $z$ direction) between $K$ and $K'$ valleys, which is non-zero under $E_z \neq 0$, cannot be fully relaxed due to missing of the relevant intervalley scatterings. Indeed, this has been observed in the spin relaxation in ML-Ge under $E_z$=5 V/nm shown in Fig. S2. From Fig. S2, under a finite $E_z$, the decay of $S_z$ of ML-Ge cannot be fitted by Eq. S2 but instead satisfies

$$S_i(t) - S_i^{\text{eq}} = \left[S_i(t_0) - S_i^{\text{eq}}\right]\left\{c * \exp\left[-\frac{t-t_0}{\tau_{s,i}^{\text{intra}}}\right] + 1 - c\right\} \times \cos\left[\omega_B(t-t_0) + \phi\right], \tag{S3}$$

with $c$ being a constant ranging from 0 to 1. The two limiting cases - $c = 0$ and $c = 1$ correspond to no relaxation and single exponential decay (if no periodic oscillations or $\omega_B = 0$), respectively. When $0 < c < 1$, a part of spin imbalance will decay out with a time constant $\tau_{s,i}^{\text{intra}}$ while the left will keep constant during the whole time.

We can further find that $c$ decreases with decreasing temperature and becomes small at low temperatures. This is because at low temperatures, most carriers are around the band edges or in the low-energy region, thus most free carriers at $K$ valley are spin-up but are spin-down in $K'$ valley due to time-reversal symmetry. Therefore, at low T, total spin imbalance is mostly the imbalance between $K$ and $K'$ valley and cannot completely decay to zero due to the missing intervalley processes.

Having the above information, we can now take the weight factor $w = \exp\left[-(1-c)/c\right]$. Thus, if spin can be fully relaxed ($c = 1$), $w = 1$ and $\eta = \left(\tau_{s,z}^{\text{inter}}\right)^{-1} / \left[\left(\tau_{s,z}^{\text{inter}}\right)^{-1} + \left(\tau_{s,z}^{\text{intra}}\right)^{-1}\right]$ will be simply determined by the ratio of $\tau_{s,z}^{\text{inter}}$ and $\tau_{s,z}^{\text{intra}}$. If intravalley scattering does not relax spin ($c = 0$), $w = 0$ and $\eta$ will be 1. This definition also ensures that if only a little part, e.g., 10% of total spin can be relaxed by intravalley scattering, $w$ is sufficiently small and $\eta$ will be close to 1. Note that $S_z$ can be fully relaxed with only intervalley scattering as we observed, so that a weigh factor is not needed for intervalley scattering.

## SIII. SPIN MIXING PARAMETER

The spin mixing parameter is defined the same as Ref. 2. Suppose the spin of a state "1" (which is the combined index of k-point and band) is highly polarized along $z$ direction. Then in general, the wavefunction of state "1" can be written as $\Psi_1(\mathbf{r}) = a_{z,1}(\mathbf{r})\alpha + b_{z,1}(\mathbf{r})\beta$, where $a$ and $b$ are the coefficients of the large and small components of the wavefunction, and $\alpha$ and $\beta$ are spinors (one up and one down for direction $z$). Define $a_{z,1}^2 = \int |a_{z,1}(\mathbf{r})|^2 d\mathbf{r}$ and $b_{z,1}^2 = \int |b_{z,1}(\mathbf{r})|^2 d\mathbf{r}$, then $a_{z,1}^2 > b_{z,1}^2$ and $b_{z,1}^2$ is just spin-mixing parameter of state "1" along direction $z$. With the definition of spin expectation value $S_{z,1}^{\exp} = s_{z,11}$, which is the diagonal element for state "1" of spin Pauli matrix along direction $z$ in Bloch basis, we have

$$a_{z,1}^2 + b_{z,1}^2 = 1, \tag{S4}$$

$$0.5\left(a_{z,1}^2 - b_{z,1}^2\right) = S_{z,1}^{\exp}, \tag{S5}$$

Therefore,

$$b_{z,1}^2 = 0.5 - S_{z,1}^{\exp}. \tag{S6}$$

## SIV. THE SPIN-FLIP MATRIX ELEMENTS AND THE SPIN-FLIP ANGLE $\theta^{\uparrow\downarrow}$

We present the detailed proof of the relation between the spin-flip matrix elements and $\theta^{\uparrow\downarrow}$ below:

**Step 1:**

For two Kramers degenerate bands, without loss of generality, the electronic states can be chosen to be one (pseudo-)spin-up and one (pseudo-)spin-down by diagonalizing spin matrix $s_z$. Suppose the first and second states are spin-up and spin-down respectively at $\mathbf{k}_1$ at $\mathbf{Q}$ valley and are spin-down and spin-up respectively at $\mathbf{k}_2$ at $-\mathbf{Q}$ valley. Thus the matrix between $\mathbf{k}_1$ and $\mathbf{k}_2$ of operator $\widehat{A}$ is

$$A_{k_1k_2}^0 = \begin{pmatrix} A_{k_1k_2}^{0,\uparrow\downarrow} & A_{k_1k_2}^{0,\uparrow\uparrow} \\ A_{k_1k_2}^{0,\downarrow\downarrow} & A_{k_1k_2}^{0,\downarrow\uparrow} \end{pmatrix}, \tag{S7}$$

According to Ref. 3, with time-reversal symmetry, the spin-flip matrix element between two states of the same band at $\mathbf{k}$ and $-\mathbf{k}$ is exactly zero. Since $\mathbf{k}_1 + \mathbf{k}_2 \approx 0$, we have $A_{k_1k_2}^{0,\uparrow\downarrow} \approx A_{k_1k_2}^{0,\downarrow\uparrow} \approx 0$ at the lowest order, so

$$A_{k_1k_2}^0 \approx \begin{pmatrix} 0 & A_{k_1k_2}^{0,\uparrow\uparrow} \\ A_{k_1k_2}^{0,\downarrow\downarrow} & 0 \end{pmatrix}. \tag{S8}$$

**Step 2:**

Moreover, the spin matrix along $z$ direction is,

$$s_{z,k}^0 = \zeta_k \hbar \begin{pmatrix} 0.5 - b_{0,k}^2 & 0 \\ 0 & b_{0,k}^2 - 0.5 \end{pmatrix}, \tag{S9}$$

where $\zeta_k$ is 1 and -1 if $\mathbf{k} = \mathbf{k}_1$ and $\mathbf{k} = \mathbf{k}_2$ respectively. $b_{0,k}^2$ is the spin-mixing parameter before the inversion symmetry being broken. If the wavefunctions are not related to heavy elements, $b_{0,k}^2$ are tiny, e.g., of order $10^{-4}$ for states near Dirac cones of germanene. Therefore,

$$s_{z,k}^0 \approx 0.5\zeta_k \hbar \begin{pmatrix} 1 & 0 \\ 0 & -1 \end{pmatrix}, \tag{S10}$$

The spin matrix along $x$ is approximately

$$s_{x,k}^{0} \approx 0.5 \begin{pmatrix} 0 & 1 \\ 1 & 0 \end{pmatrix}. \tag{S11}$$

Now suppose the inversion symmetry is broken, which induces internal magnetic fields $\mathbf{B}_k^{\mathrm{in}}$.
Without loss of generality, we assume

$$\mathbf{B}_{k_1}^{\mathrm{in}} = B_1 \left(\sin\theta_{k_1k_2}^{\uparrow\downarrow}, 0, \cos\theta_{k_1k_2}^{\uparrow\downarrow}\right), \tag{S12}$$

$$\mathbf{B}_{k_2}^{\mathrm{in}} = B_2 \left(0, 0, -1\right). \tag{S13}$$

Indeed $\theta_{k_1k_2}^{\uparrow\downarrow}$ is the angle between $-\mathbf{B}_{k_1}^{\mathrm{in}}$ and $\mathbf{B}_{k_2}^{\mathrm{in}}$.
The perturbed Hamiltonians $H_k^{\mathrm{ISB}} = \mu_B g_e \mathbf{B}_k^{\mathrm{in}} \cdot \mathbf{s}_k^0$ are

$$H_{k_1}^{\mathrm{ISB}} \approx 0.5\hbar\mu_B g_e B_1 \begin{pmatrix} \cos\theta_{k_1k_2}^{\uparrow\downarrow} & \sin\theta_{k_1k_2}^{\uparrow\downarrow} \\ \sin\theta_{k_1k_2}^{\uparrow\downarrow} & -\cos\theta_{k_1k_2}^{\uparrow\downarrow} \end{pmatrix}, \tag{S14}$$

$$H_{k_2}^{\mathrm{ISB}} \approx 0.5\hbar\mu_B g_e B_2 \begin{pmatrix} -1 & 0 \\ 0 & 1 \end{pmatrix}. \tag{S15}$$

According to first-order degenerate perturbation theory, the new eigenvectors are obtained by diagonalizing $H'$.
The eigenvectors $U$ are

$$U_{k_1} = \begin{pmatrix} \cos\left(\theta_{k_1k_2}^{\uparrow\downarrow}/2\right) & -\sin\left(\theta_{k_1k_2}^{\uparrow\downarrow}/2\right) \\ \sin\left(\theta_{k_1k_2}^{\uparrow\downarrow}/2\right) & \cos\left(\theta_{k_1k_2}^{\uparrow\downarrow}/2\right) \end{pmatrix}, \tag{S16}$$

$$U_{k_2} = \begin{pmatrix} 1 & 0 \\ 0 & 1 \end{pmatrix}. \tag{S17}$$

**Step 3:**
Therefore, the new matrix of operator $\widehat{A}$,

$$A_{k_1k_2} = U_{k_1}^{\dagger} A_{k_1k_2}^{0} U_{k_2} \tag{S18}$$

$$\approx \begin{pmatrix} \sin\left(\theta_{k_1k_2}^{\uparrow\downarrow}/2\right) A_{k_1k_2}^{0,\downarrow\downarrow} & A_{k_1k_2}^{0,\uparrow\uparrow} \\ A_{k_1k_2}^{0,\downarrow\downarrow} & -\sin\left(\theta_{k_1k_2}^{\uparrow\downarrow}/2\right) A_{k_1k_2}^{0,\uparrow\uparrow} \end{pmatrix}. \tag{S19}$$

To obtain the above equation, we use the approximate relation $\cos\left(\theta_{k_1k_2}^{\uparrow\downarrow}/2\right) \approx 1$ and the resulting relation $A_{k_1k_2}^{\downarrow\downarrow} \approx A_{k_1k_2}^{0,\downarrow\downarrow}$. Therefore, $A_{k_1k_2}^{\uparrow\downarrow} \approx \sin\left(\theta_{k_1k_2}^{\uparrow\downarrow}/2\right) A_{k_1k_2}^{0,\downarrow\downarrow} \approx \sin\left(\theta_{k_1k_2}^{\uparrow\downarrow}/2\right) A_{k_1k_2}^{\downarrow\downarrow}$.

Moreover, since $\mathbf{k}_1$ and $\mathbf{k}_2$ are near $\mathbf{Q}$ and $-\mathbf{Q}$, the spin-conserving matrix elements are approximately $A_{Q,-Q}^{0,\uparrow\uparrow}$ or $A_{Q,-Q}^{\uparrow\uparrow}$ ($A_{Q,-Q}^{\uparrow\uparrow} \approx A_{Q,-Q}^{\downarrow\downarrow}$ due to time-reversal symmetry[3]), i.e., $A_{k_1k_2}^{\downarrow\downarrow} \approx A_{k_1k_2}^{\uparrow\uparrow} \approx A_{Q,-Q}^{\uparrow\uparrow}$. Therefore, we further have

$$A_{k_1k_2} \approx A_{Q,-Q}^{\uparrow\uparrow} \begin{pmatrix} \sin\left(\theta_{k_1k_2}^{\uparrow\downarrow}/2\right) & 1 \\ 1 & -\sin\left(\theta_{k_1k_2}^{\uparrow\downarrow}/2\right) \end{pmatrix}. \tag{S20}$$

So $A_{k_1k_2}^{\uparrow\downarrow} \approx \sin\left(\theta_{k_1k_2}^{\uparrow\downarrow}/2\right) A_{Q,-Q}^{\uparrow\uparrow}$. We then have $\left|A_{k_1k_2}^{\uparrow\downarrow}\right|^2 \approx \sin^2\left(\theta_{k_1k_2}^{\uparrow\downarrow}/2\right) \left|A_{Q,-Q}^{\uparrow\uparrow}\right|^2$.

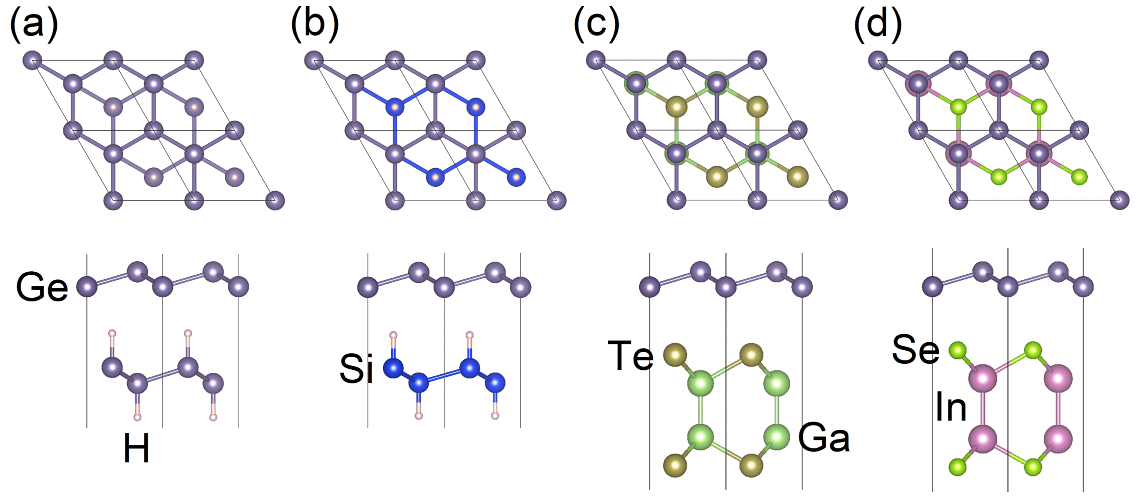


FIG. S3. Top and side views of 2×2 supercells of ML-Ge on (a) GeH, (b) SiH, (c) GaTe and (d) InSe substrates.

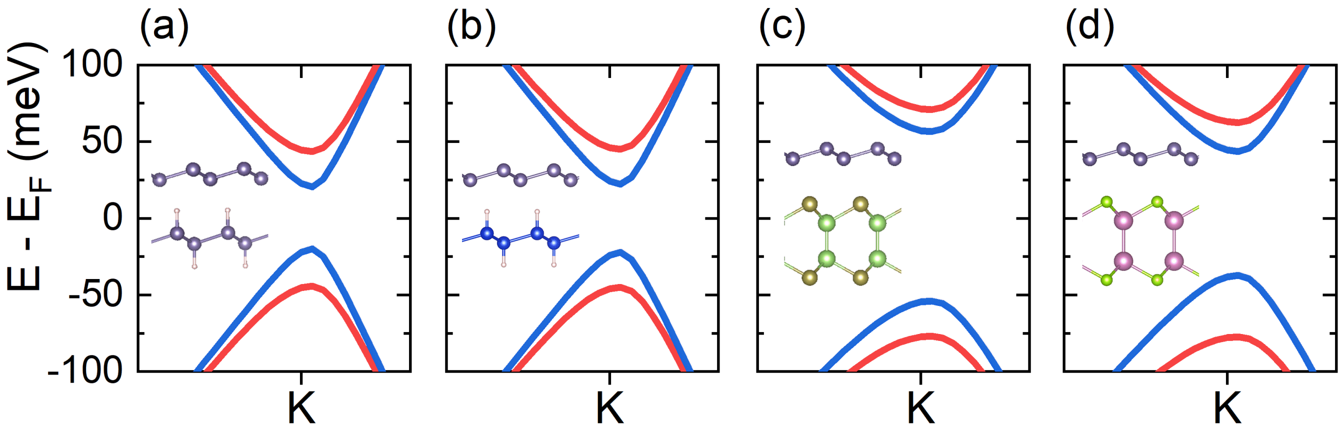


FIG. S4. Band structures around a Dirac cone of ML-Ge on (a) GeH, (b) SiH, (c) GaTe and (d) InSe substrates. The red and blue bands correspond to spin-up and spin-down bands.

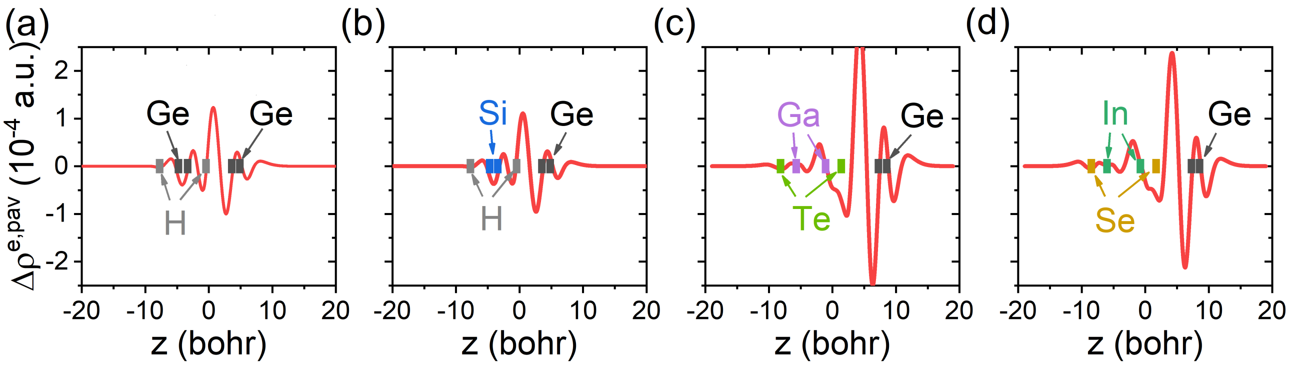


FIG. S5. The planar averaged differential electron charge density $\Delta\rho^{e,\mathrm{pav}}(z)$ of ML-Ge on (a) GeH, (b) SiH, (c) GaTe and (d) InSe substrates. "pav" means the charge density is averaged over the values on a $xy$ plane. $\Delta\rho^{e} = \rho^{e,\mathrm{ML-GE-Sub}} - \rho^{e,\mathrm{ML-GE}} - \rho^{e,\mathrm{Sub}}$, where $\rho^{e,\mathrm{ML-GE-Sub}}$, $\rho^{e,\mathrm{ML-GE}}$ and $\rho^{e,\mathrm{Sub}}$ means the charge density of ML-Ge on a substrate, ML-Ge and the substrate respectively.

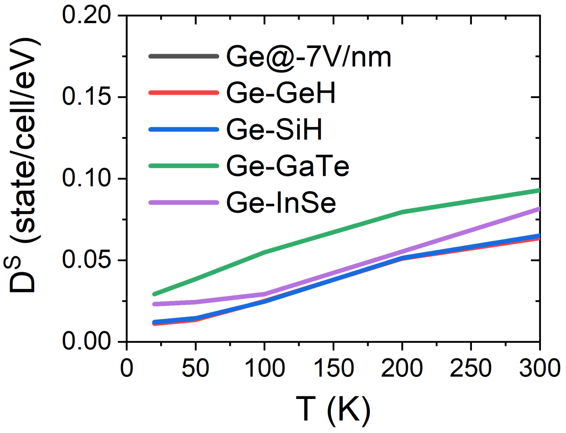


FIG. S6. The scattering density of state $D^S$ (Eq. 9 in "Method" section in the main text) of intrinsic ML-Ge systems as a function of $T$. The black curve overlaps with red and blue curves.

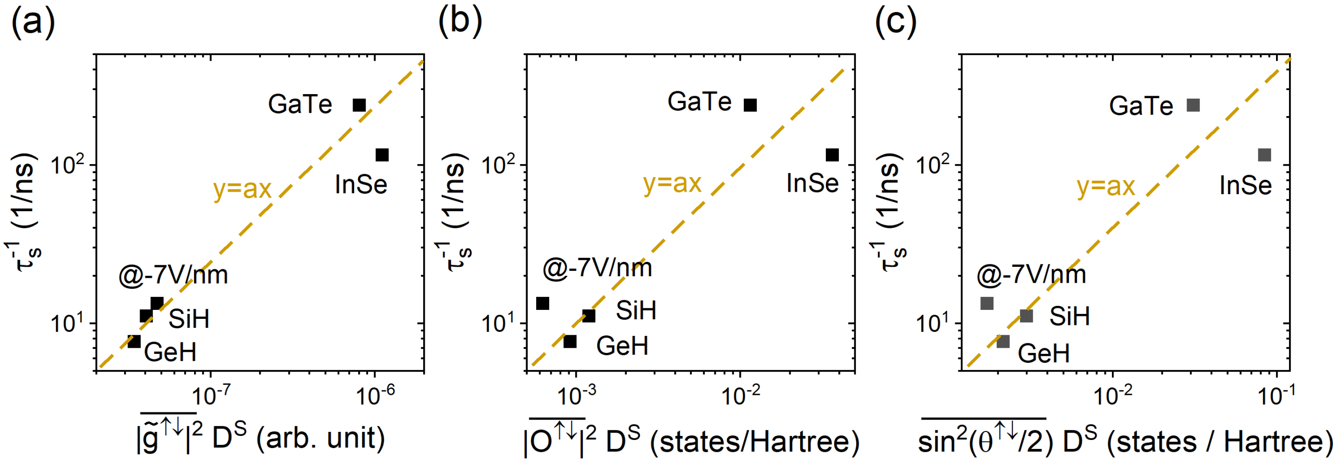


FIG. S7. The relation between $\tau_s^{-1}$ and the averaged modulus square of spin-flip e-ph matrix elements $\overline{|\tilde{g}^{\uparrow\downarrow}|^2}$, of spin-flip overlap matrix elements $\overline{|o^{\uparrow\downarrow}|^2}$ and $\overline{\sin^2\left(\theta^{\uparrow\downarrow}/2\right)}$ multiplied by the scattering density of states $D^S$ at 300 K. See the definition of $\overline{|\tilde{g}^{\uparrow\downarrow}|^2}$, $\overline{|o^{\uparrow\downarrow}|^2}$ and $D^S$ in Eq. 8, 19 and 9 in the main text respectively. $\theta^{\uparrow\downarrow}$ is the spin-flip angle between two electronic states. For two states $(k,n)$ and $(k',n')$ with opposite spin directions, $\theta^{\uparrow\downarrow}$ is the angle between $-\mathbf{S}_{kn}^{\mathrm{exp}}$ and $\mathbf{S}_{k'n'}^{\mathrm{exp}}$. $\overline{\sin^2\left(\theta^{\uparrow\downarrow}/2\right)}$ is defined in Eq. 24 in the main text. The variation of $D^S$ among different substrates is at most three times, much weaker than the variations of $\tau_s^{-1}$ and other quantities shown here. The characteristic transition energy $\omega_c$ is simply taken as half of the maximum phonon frequency, ~10 meV, of ML-Ge at 300 K, since at this temperature all phonon modes contribute to spin relaxation.

## SV. THE FLUCTUATION AMPLITUDE OF $B_z^{\mathrm{in}}$ AND $\left|B_z^{\mathrm{in}}\right|$

For two bands splitting by the k-dependent internal magnetic field $\mathbf{B}_k^{\mathrm{in}}$ (defined Eq. 21 in the main text), the fluctuation amplitude (among different k-points) of the z component of $\mathbf{B}^{\mathrm{in}}$ - $\Delta B_z^{\mathrm{in}}$ is defined as:

$$\Delta B_z^{\mathrm{in}} = \frac{\sum_{kn}\left(-f'_{kn}\right)\left(B_{k,z}^{\mathrm{in}} - \overline{B_{k,z}^{\mathrm{in}}}\right)^2}{\sum_{kn}\left(-f'_{kn}\right)}, \tag{S21}$$

$$\overline{B_{k,z}^{\mathrm{in}}} = \frac{\sum_{kn}\left(-f'_{kn}\right)B_{k,z}^{\mathrm{in}}}{\sum_{kn}\left(-f'_{kn}\right)}, \tag{S22}$$

where $f'_{kn}$ is the derivative of the Fermi-Dirac distribution function of the state $(k,n)$. Due to time reversal symmetry, $\overline{B_{k,z}^{\mathrm{in}}} \equiv 0$.

The fluctuation amplitude of $\left|B_z^{\mathrm{in}}\right|$ - $\Delta\left|B_z^{\mathrm{in}}\right|$ is

$$\Delta\left|B_z^{\mathrm{in}}\right| = \frac{\sum_{kn}\left(-f'_{kn}\right)\left(\left|B_{k,z}^{\mathrm{in}}\right| - \overline{\left|B_{k,z}^{\mathrm{in}}\right|}\right)^2}{\sum_{kn}\left(-f'_{kn}\right)}, \quad \text{(S23)}$$

$$\overline{\left|B_z^{\mathrm{in}}\right|} = \frac{\sum_{kn}\left(-f'_{kn}\right)\left|B_{k,z}^{\mathrm{in}}\right|}{\sum_{kn}\left(-f'_{kn}\right)}. \quad \text{(S24)}$$

| Substrate | $\Delta B_z^{\mathrm{in}}$ (Tesla) | $\Delta\lvert B_z^{\mathrm{in}}\rvert$ (Tesla) | $t_\Omega$ (ps) | $\tau_{s,x}$ (ps) | $\tau_{s,z}$ (ps) |
|---|---|---|---|---|---|
| @0 V/nm | 0 | 0 | $\infty$ | 104 | 74000 |
| @-7 V/nm | 180 | 17.5 | 0.186 | 0.49 | 109000 |
| GeH | 179 | 17.3 | 0.188 | 0.51 | 92000 |
| SiH | 180 | 16.2 | 0.187 | 0.54 | 2400 |
| GaTe | 117 | 7.8 | 0.298 | 0.73 | 2900 |
| InSe | 329 | 15.0 | 0.106 | 0.45 | 1100 |

TABLE S1. $\Delta B_z^{\mathrm{in}}$, $\Delta|B_z^{\mathrm{in}}|$, the Larmor precession period $t_\Omega = 2\pi/\Omega$, the in-plane spin lifetime $\tau_{s,x}$ and the out-of-plane spin lifetime $\tau_{s,z}$ of ML-Ge at $E_z = -7$ V/nm and different substrates at 50 K. $\Delta B_z^{\mathrm{in}}$ is the fluctuation amplitude (among different k-points) of the $z$ component of internal magnetic field ($\mathbf{B}^{\mathrm{in}} \equiv \left(B_x^{\mathrm{in}}, B_y^{\mathrm{in}}, B_z^{\mathrm{in}}\right)$ defined in Eq. 21 in the main text) and is defined in Eq. S21. $\Delta|B_z^{\mathrm{in}}|$ is the fluctuation amplitude of $|B_z^{\mathrm{in}}|$ defined in Eq. S23 and is also the fluctuation amplitude of $B_z^{\mathrm{in}}$ within the same valley, since $B_z^{\mathrm{in}}$ at k-points within the same valley have the same sign. $t_\Omega = 2\pi/\Omega$ is the Larmor precession period extracted from time evolution of spin observable $S_x$ for spin decay along the $x$ direction. When spin relaxation is dominated by DP or free induction decay mechanism[4], $\Delta B_z^{\mathrm{in}}$ and $\Delta|B_z^{\mathrm{in}}|$ are related to spin relaxation. When intervalley transitions are much slower than in-plane spin relaxation (which is true at low $T$), in-plane spin relaxation within one valley is almost independent from that in the other valley, so that in-plane spin relaxation is only determined by $\Delta|B_z^{\mathrm{in}}|$ but not $\Delta B_z^{\mathrm{in}}$. While $\Delta B_z^{\mathrm{in}}$ can be important to in-plane spin relaxation if intervalley spin-conserving transitions are allowed.

---


* jxu153@ucsc.edu
† yuanping@ucsc.edu



1 J. Xu, A. Habib, R. Sundararaman, and Y. Ping, Phys. Rev. B **104**, 184418 (2021).
2 J. Xu, H. Takenaka, A. Habib, R. Sundararaman, and Y. Ping, Nano Lett. **21**, 9594 (2021).
3 Y. Yafet, in *Solid state physics*, Vol. 14 (Elsevier, 1963) pp. 1–98.
4 M. Wu, J. Jiang, and M. Weng, Phys. Rep. **493**, 61 (2010).
